# Supplementary material for: Who Shares Fake News? Uncovering Insights from Social Media Users' Post Histories
Source: arXiv:2203.10560 source file (2024-07-22)
Supplement: Supplementary file 1 [file WebAppendix_Newsheadlines.tex]

\setcounter{table}{0}
\setcounter{figure}{0}

\setlength{\baselineskip}{21pt plus.2pt}

\section*{Web Appendix O - News Article Headlines}

\vspace{8pt}

\begin{table}[htbp]
\begin{tabular}{ll}
\begin{tabular}[c]{@{}l@{}}Status\\ (Fake = 1)\end{tabular} & News Headline \\
\hline\hline
1 & For Native Peoples, Thanksgiving Isn’t A Celebration. It’s A National Day Of Mourning \\
0 & Nevermind' baby sues Nirvana, alleging album cover was child porn \\
1 & \begin{tabular}[c]{@{}l@{}}Virginia man arrested for having Minecraft worlds that were exact \\ replicas of classified U.S. military bases.\end{tabular} \\
0 & Brazilian Footballer Charged with Attempted Murder after Kicking Referee in the Head. \\
0 & Guns Are Banned during Trump’s Upcoming Speech at the NRA Conference \\
1 & \begin{tabular}[c]{@{}l@{}}Rep. Randy Fine of Florida’s House of Representatives tweeted: \\ “Elementary school children is a small sacrifice that I’m willing \\ to make for the Second Amendment.”\end{tabular} \\
0 & \begin{tabular}[c]{@{}l@{}}Bill Clinton was photographed with Jeffrey Epstein and Ghislaine Maxwell at the \\ White House during his time as commander in chief\end{tabular} \\
1 & On May 22: WHO Will Have Authority to Lock down All of America.
\end{tabular}
\end{table}
